# Supplementary material for: $\mathcal{P}^2$: Combining pressure and electrochemistry to synthesize superhydrides
Source: arXiv:2007.15613 source file (2020-10-20)
Supplement: Supplementary file 1 [file SI.pdf]

# Supplementary Information:
# $\mathscr{P}^2$: Combining pressure and electrochemistry to synthesize superhydrides

Pin-Wen Guan[1], Russell J. Hemley[2,3], Venkatasubramanian Viswanathan[1,4]

[1]*Department of Mechanical Engineering, Carnegie Mellon University, Pittsburgh, Pennsylvania 15213, USA*

[2]*Department of Physics, University of Illinois at Chicago, Chicago, IL 60607 USA*

[3]*Department of Chemistry, University of Illinois at Chicago, Chicago, IL 60607 USA*

[4]*Department of Physics, Carnegie Mellon University, Pittsburgh, Pennsylvania 15213, USA*

**This PDF includes:**

Supplementary Figures 1-11.

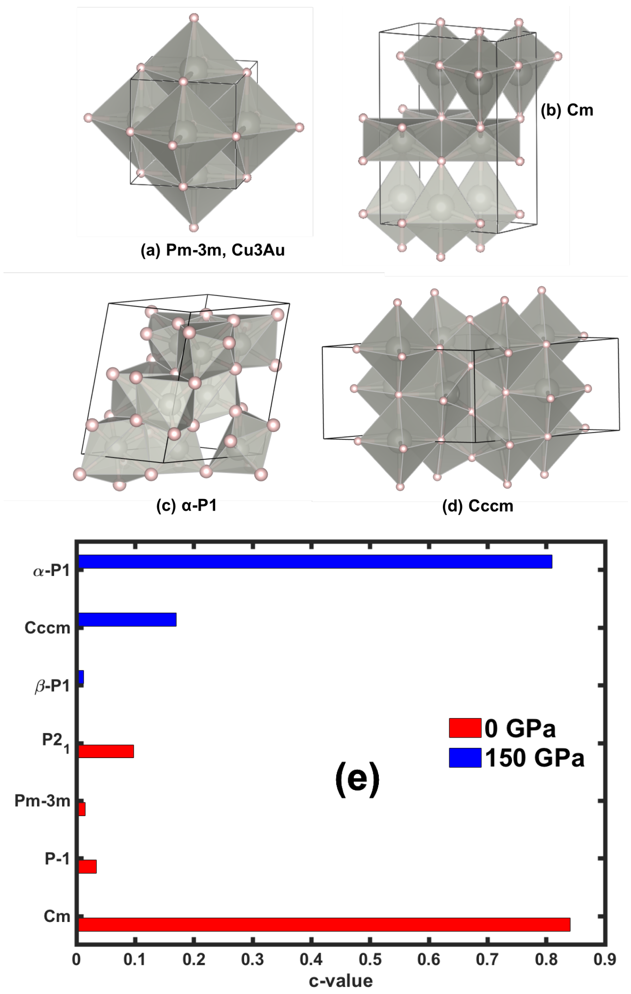


**Supplementary Figure 1:** Crystal structures of $Pd_3H_4$: (a) $Pm\bar{3}m$ (b) $Cm$ and (c) $\alpha - P1$ (d) $Cccm$. In the $Pm\bar{3}m$ structure, the Pd atom is octahedrally coordinated, whereas in the $Cm$ structure, the Pd atom has two different coordinations, with 5 and 6 neighboring H atoms respectively. The Pd atom in the low-symmetry $\alpha - P1$ structure has on average 7.11 neighboring H atoms. (d) c-values of $Pd_3H_4$ at 0 GPa and 150 GPa calculated by BEEF. The most probable structure has the $Cm$ space group, with $Pm\bar{3}m$ among the probable structures. At 150 GPa, $\alpha - P1$ structure is calculated to be the most probable.

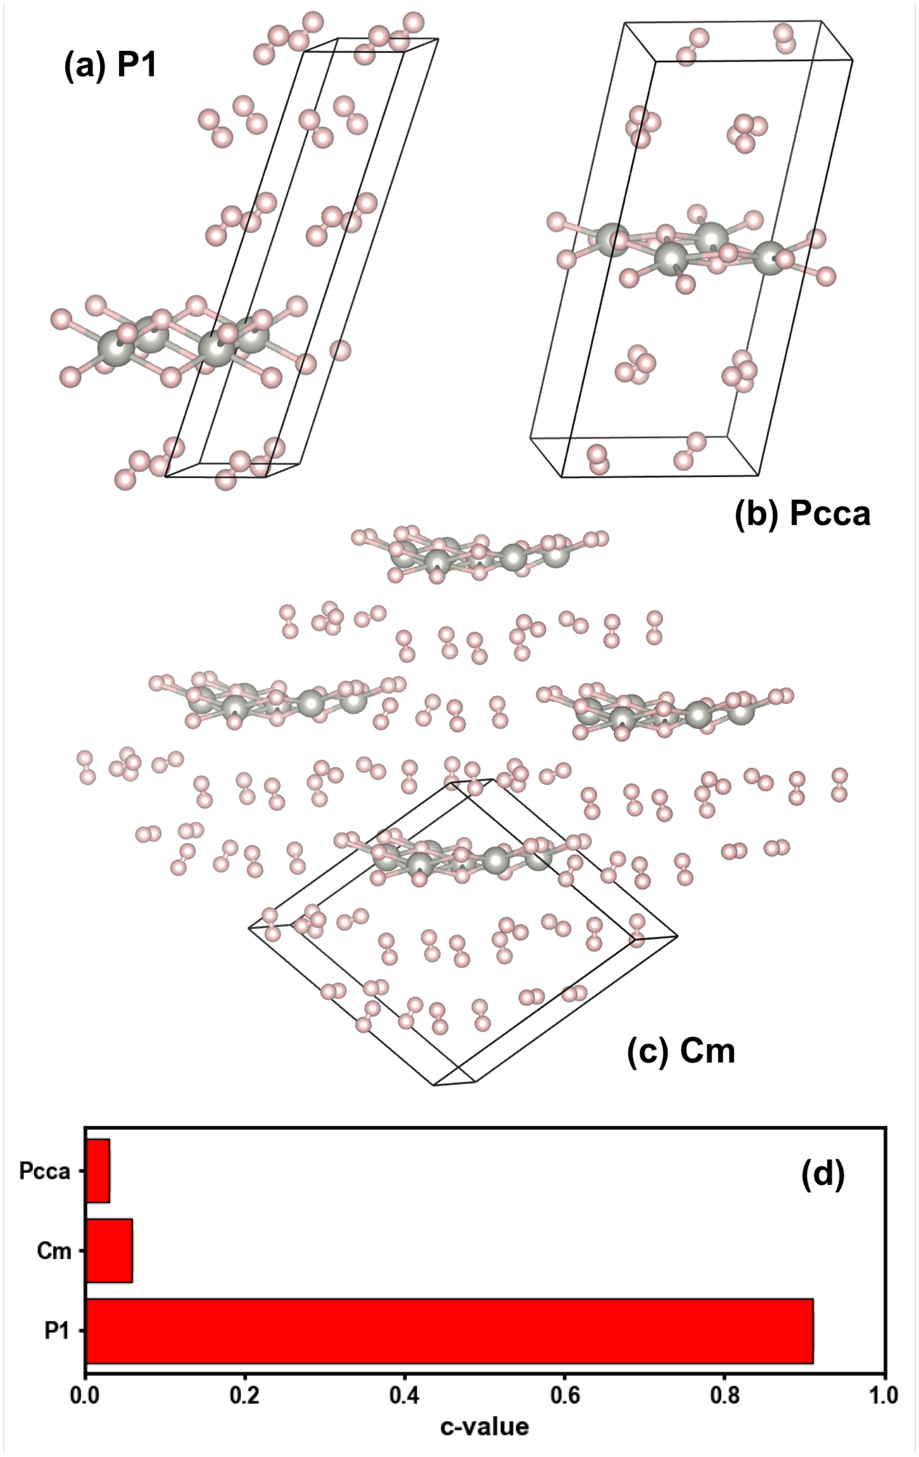


**Supplementary Figure 2:** Crystal structures of probable ground states of PdH8 at 0 GPa: (a) *P*1 (b) *Pcca* (c) *Cm*. (d) Ground states with c-values of $PdH_8$ at 0 GPa calculated by BEEF. The most probable structure has the *P*1 space group.

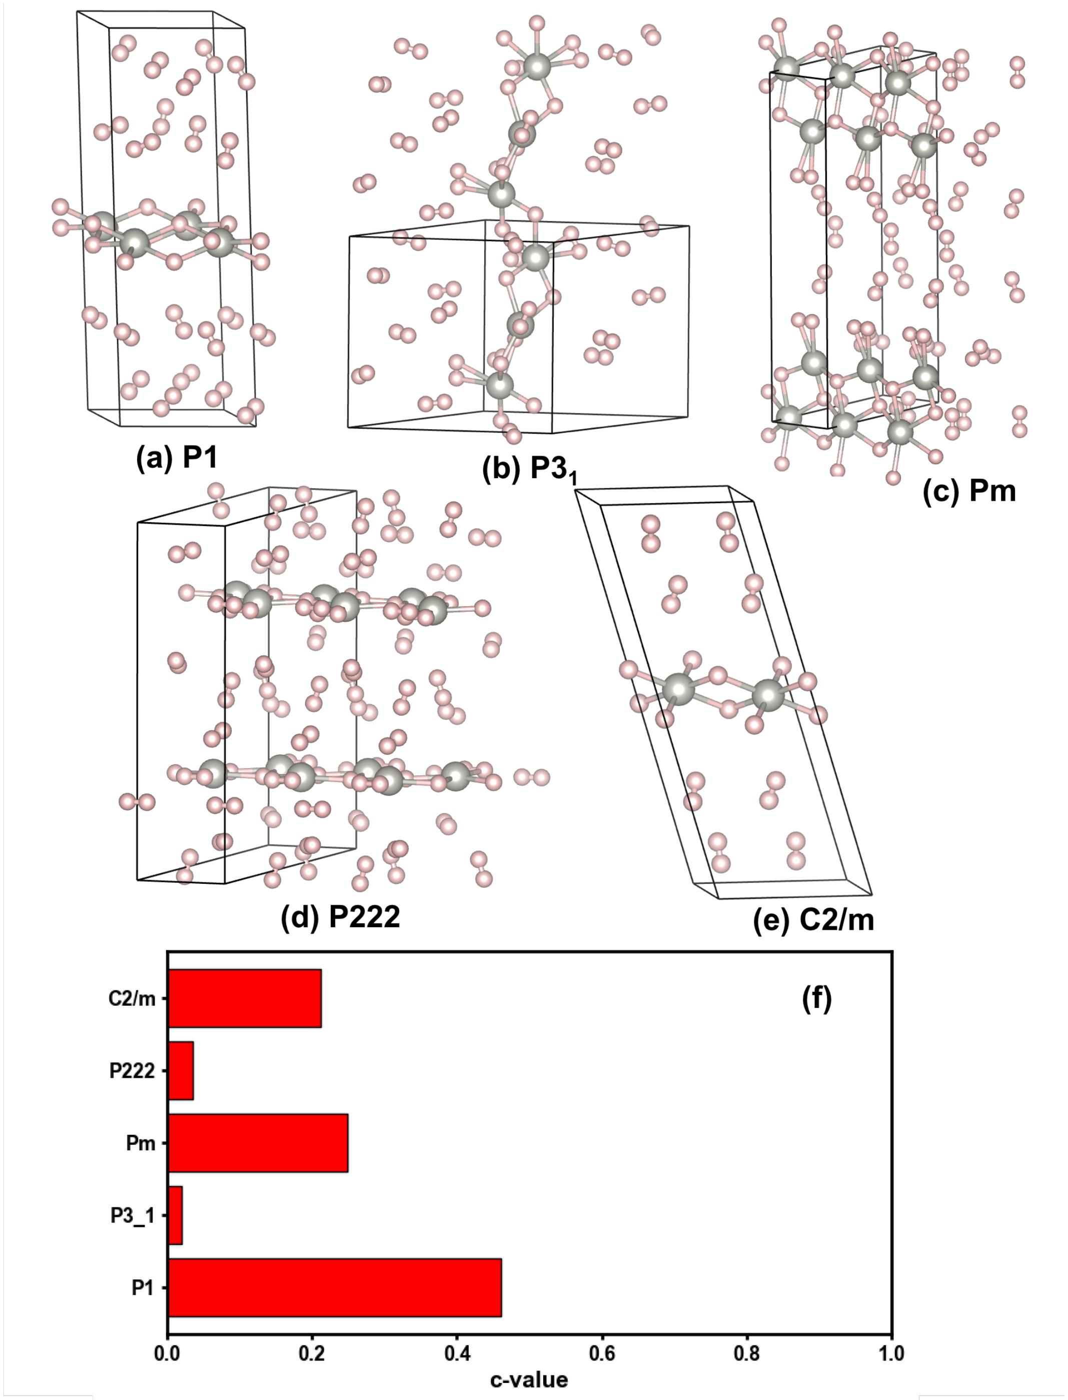


**Supplementary Figure 3:** Crystal structures of probable ground states of PdH10 at 0 GPa: (a) $P1$ (b) $P3_1$ (c) $Pm$ (d) $P222$ (e) $C2/m$. (f) Ground states with c-values of $PdH_{10}$ at 0 GPa calculated by BEEF. The most probable structure has the $P1$ space group.

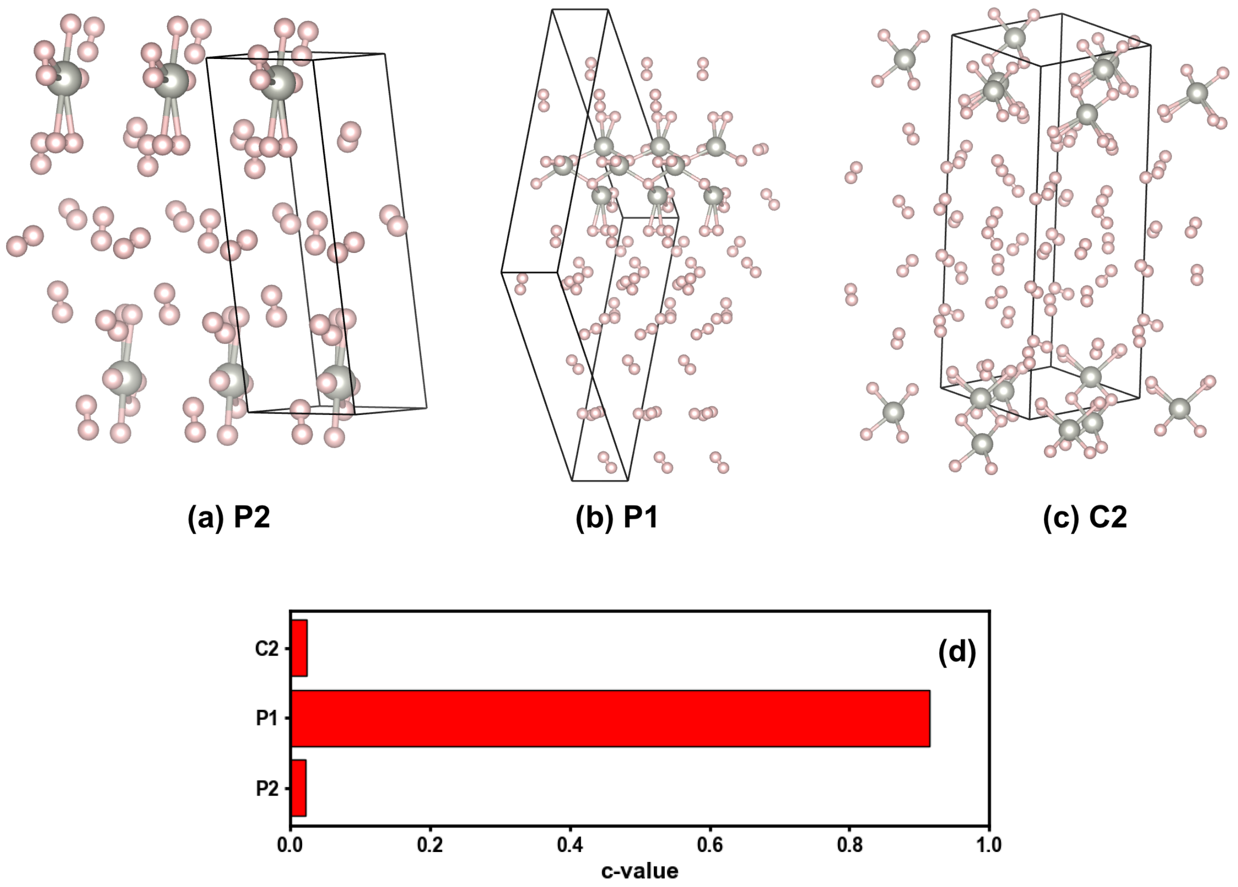


**Supplementary Figure 4:** Crystal structures of probable ground states of PdH12 at 0 GPa: (a) *P*2 (b) *P*1 (c) *C*2. (d) Ground states with c-values of $PdH_{12}$ at 0 GPa calculated by BEEF. The most probable structure has the *P*1 space group.

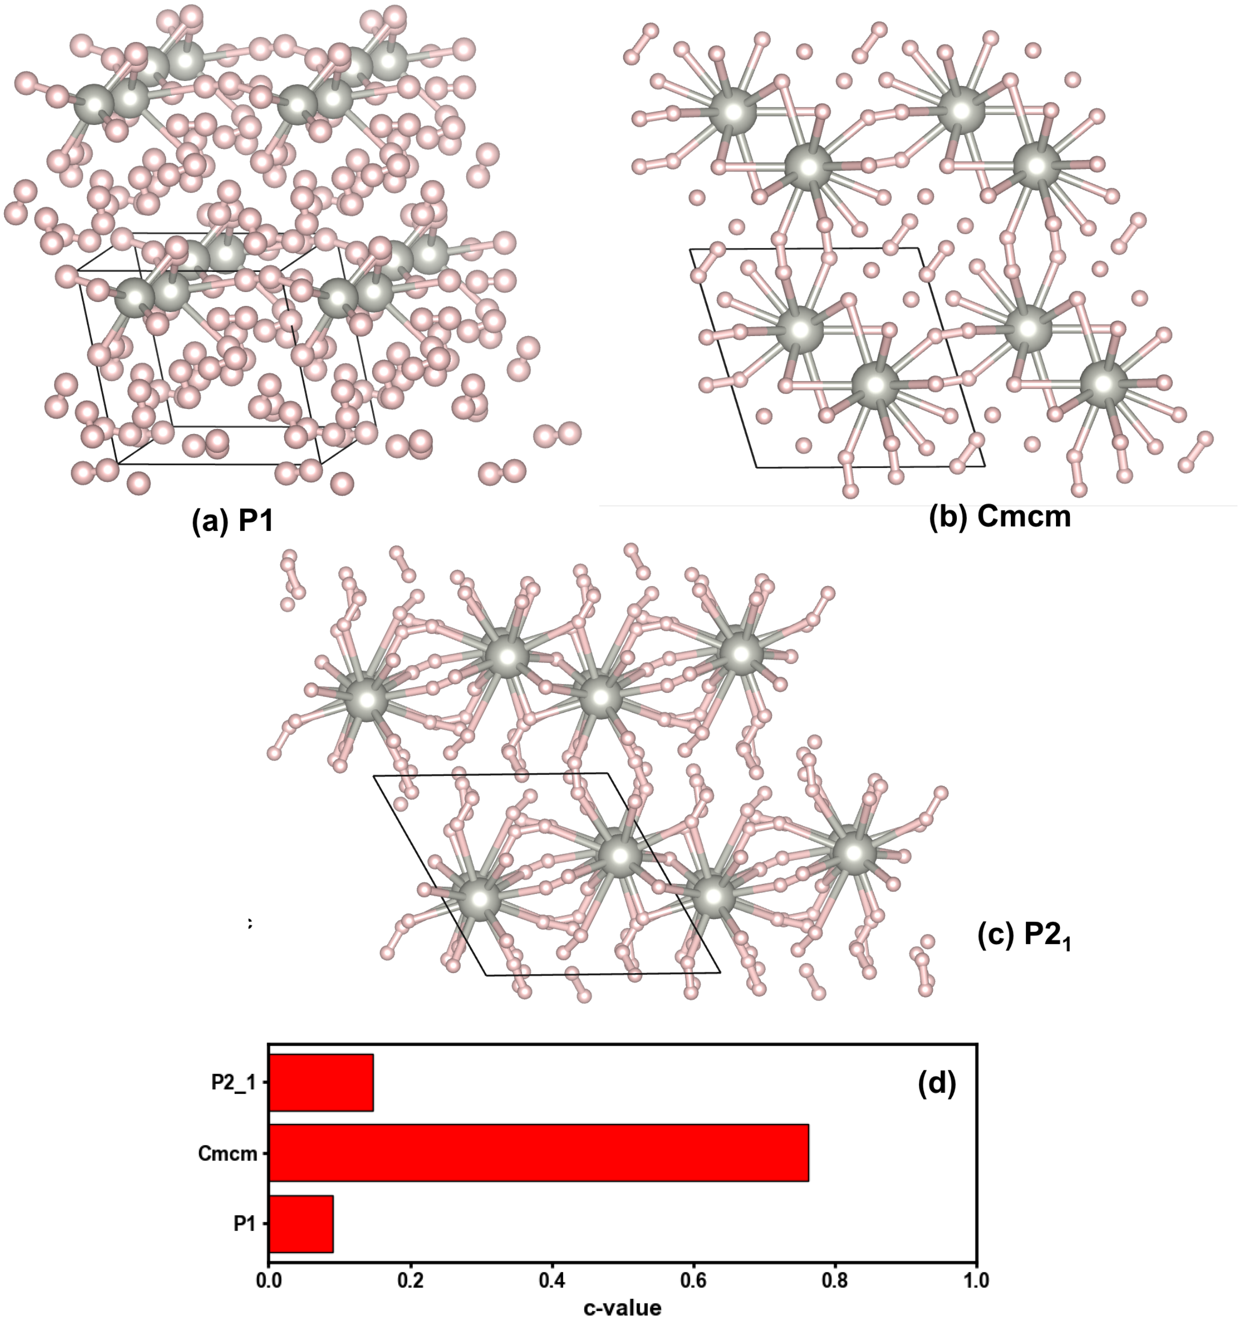


**Supplementary Figure 5:** Crystal structures of probable ground states of PdH12 at 150 GPa: (a) P1 (b) Cmcm (c) P$2_1$. (d) Ground states with c-values of $PdH_{12}$ at 150 GPa calculated by BEEF. The most probable structure has the Cmcm space group.

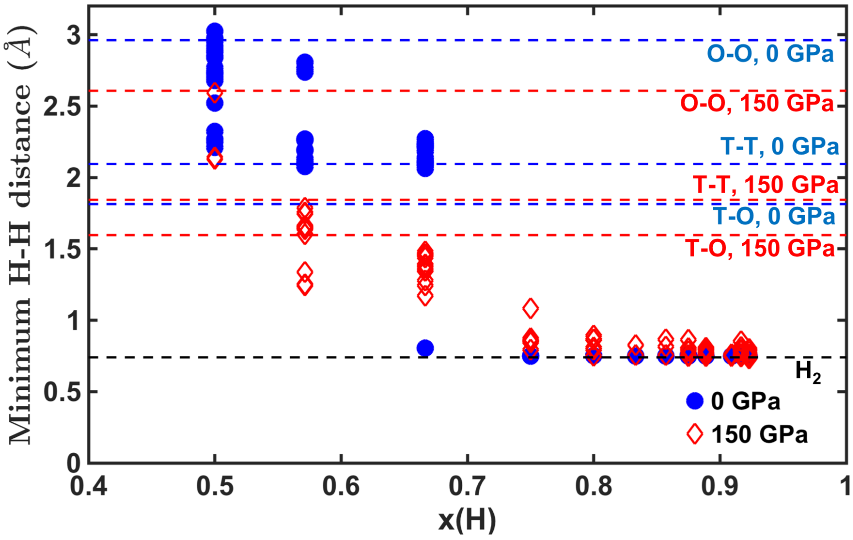


**Supplementary Figure 6:** Distribution of the minimum H-H distances of the low enthalpy structures at zero pressure and 150 GPa. The black dashed line represents the H-H distance in $H_2$ (0.74 Å).

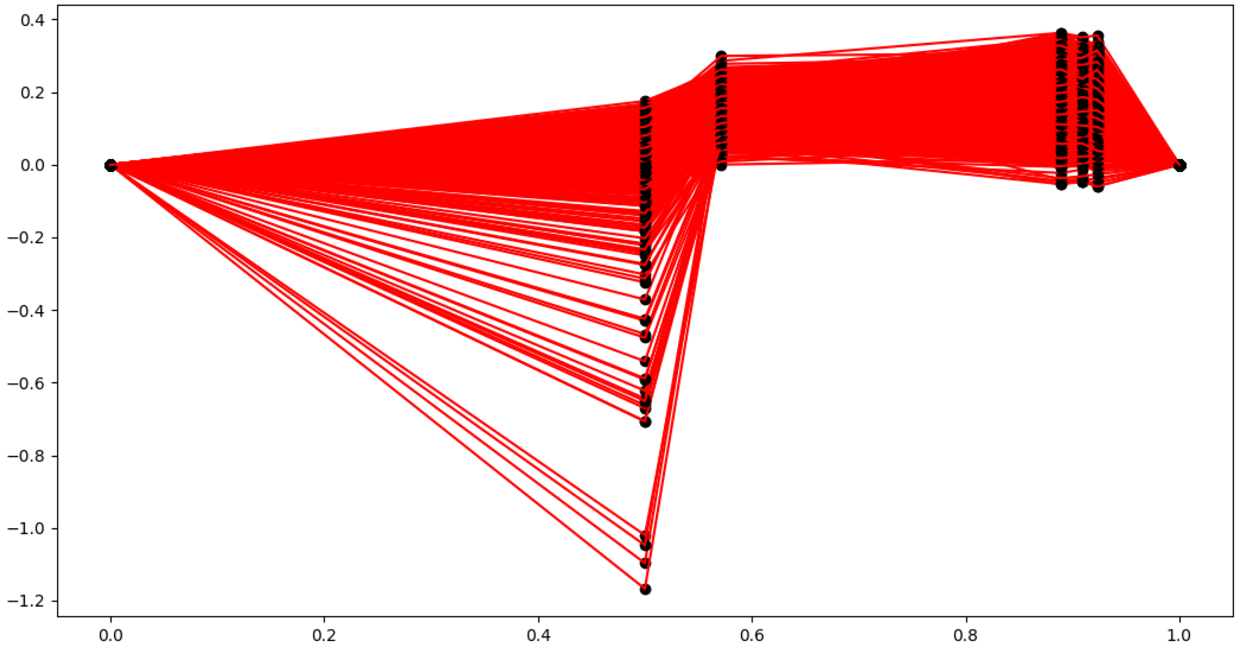


**Supplementary Figure 7:** Enthalpy convex hull of Pd-H at 0 GPa by BEEF, consisting of results from 2000 different functionals. For most functionals, Pd superhydrides are unstable against PdH and $H_2$.

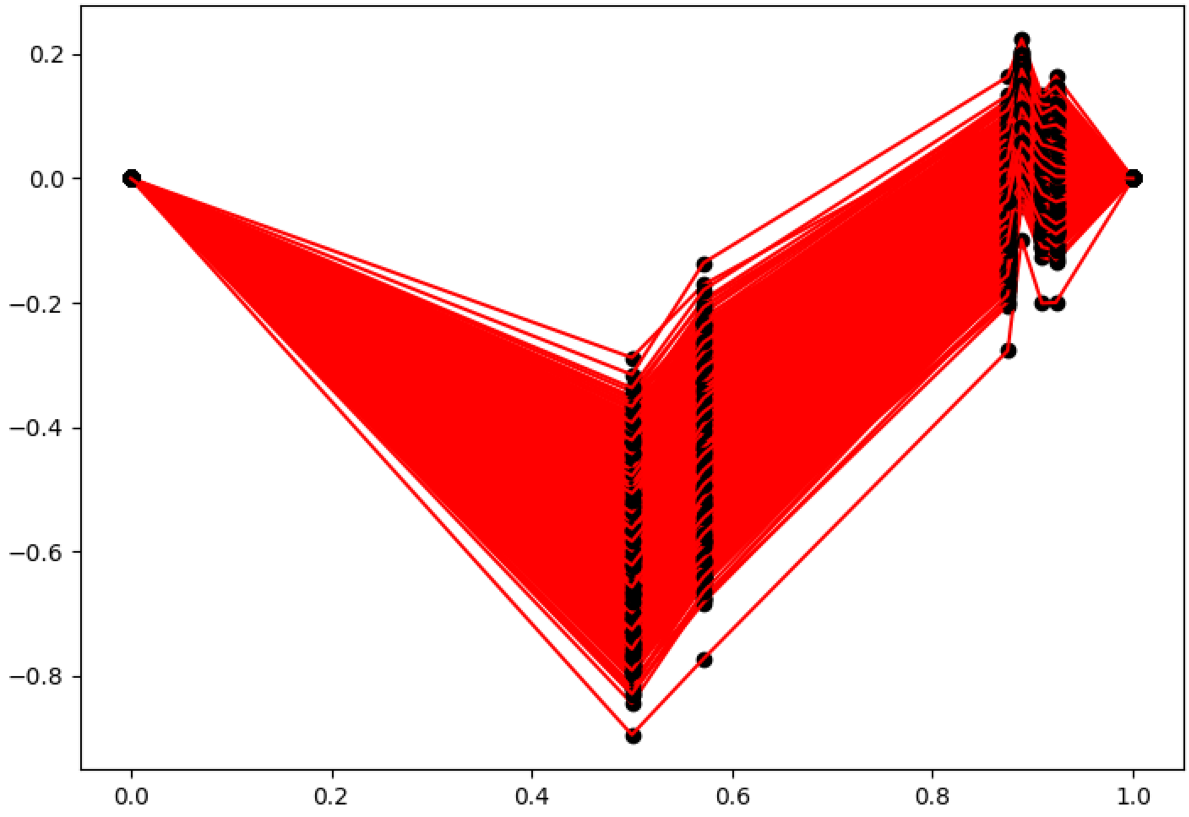


**Supplementary Figure 8:** Enthalpy convex hull of Pd-H at 150 GPa by BEEF, consisting of results from 2000 different functionals. For most functionals, Pd superhydrides are unstable against PdH and $H_2$.

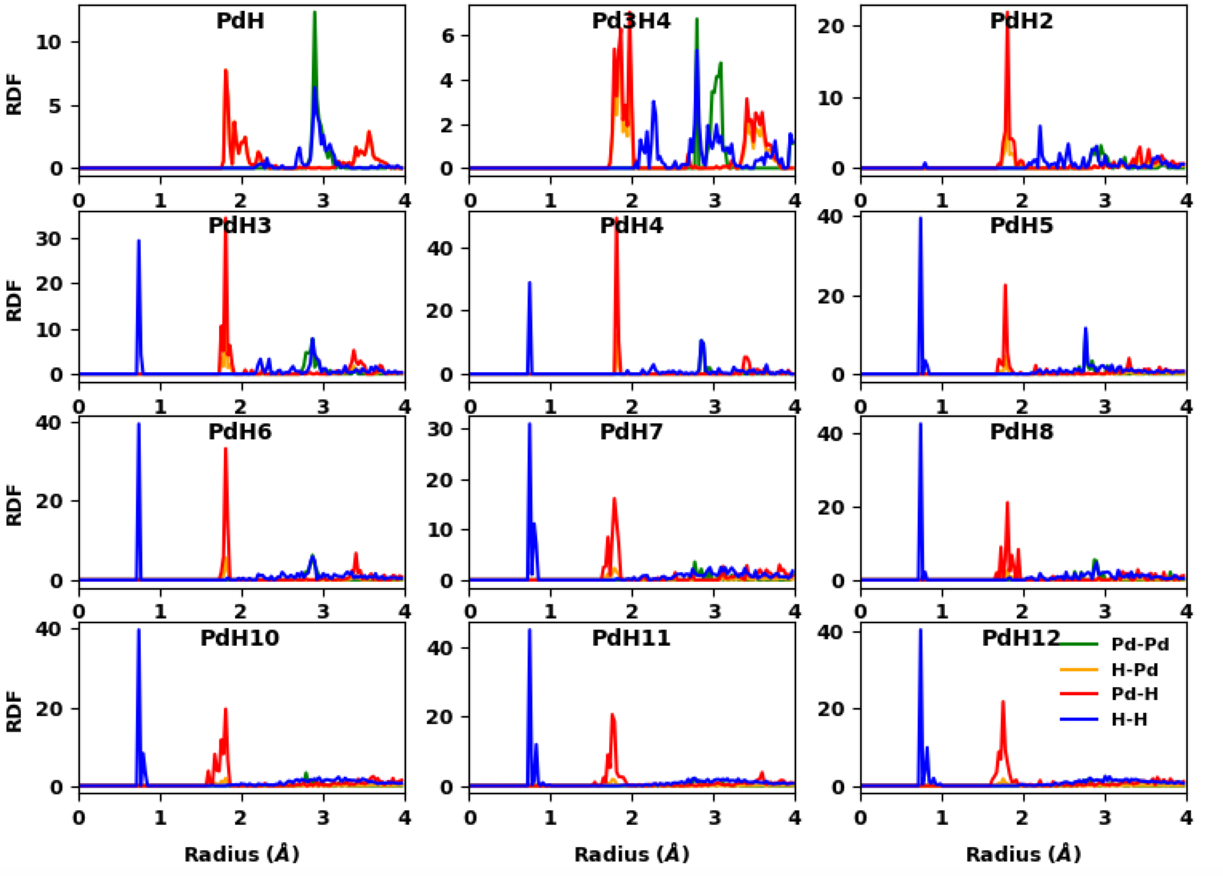


**Supplementary Figure 9:** Radial Distribution Function (RDF) of low enthalpy structures of PdHn under 0 GPa.

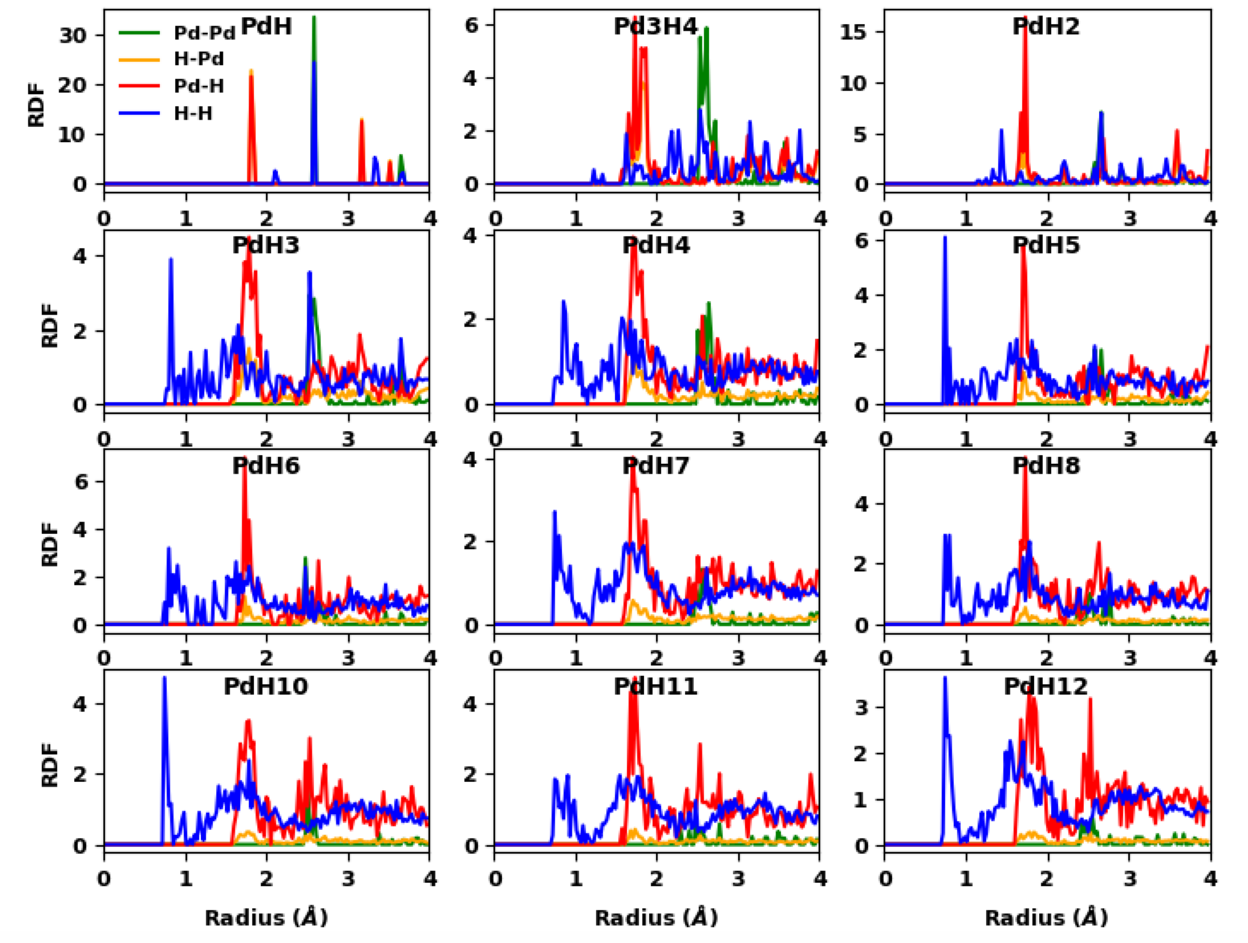


**Supplementary Figure 10:** Radial Distribution Function (RDF) of low enthalpy structures of PdHn under 150 GPa.

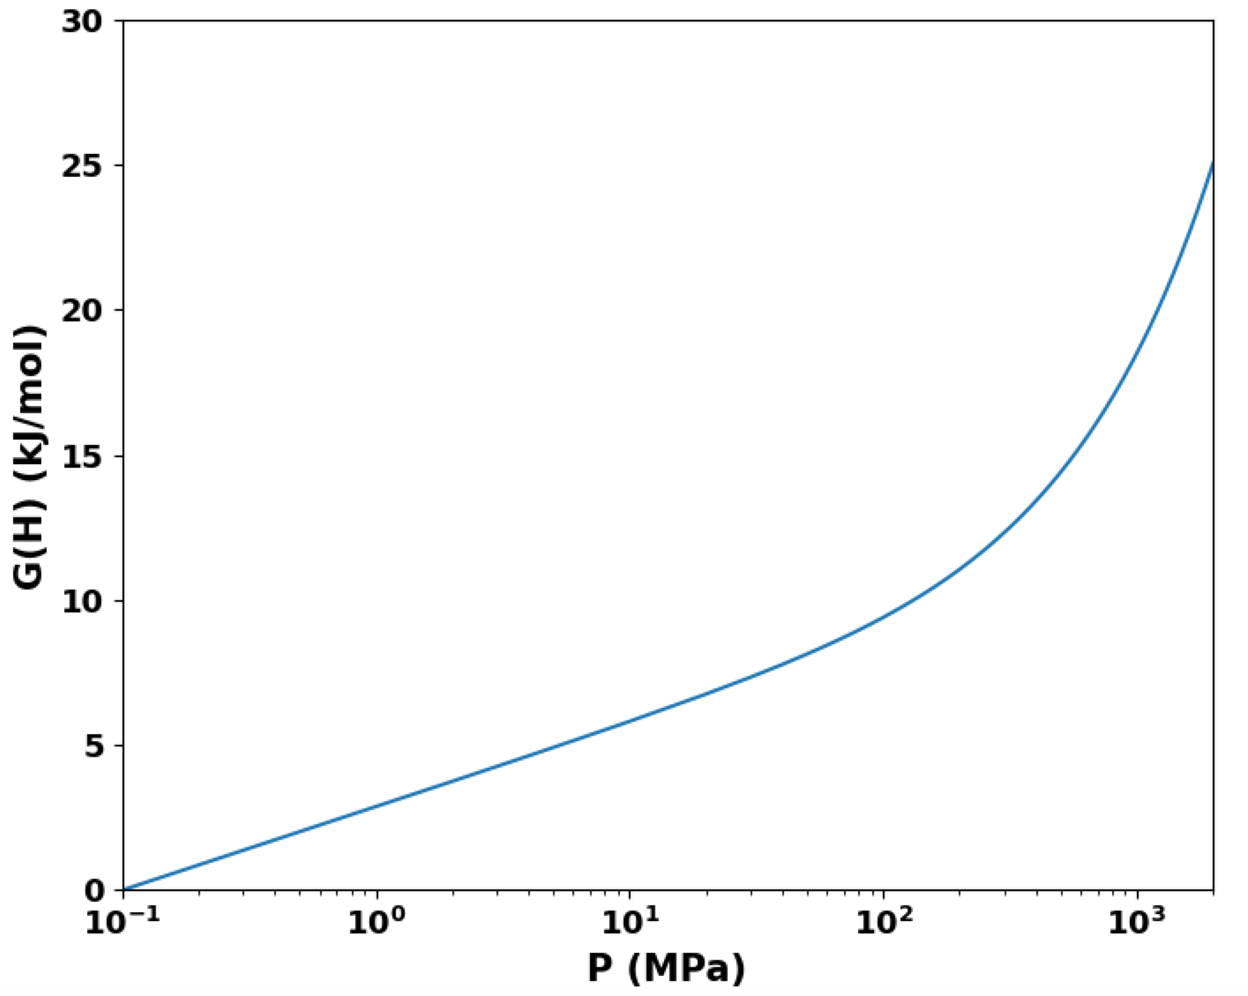


**Supplementary Figure 11:** Molar Gibbs energy of H as a function of pressure at 300 K, with its value under 1 atm (0.1 MPa) as the reference.
